# Supplementary material for: A latent process model for monitoring progress towards hard-to-measure targets, with applications to mental health and online educational assessments
Source: arXiv:2305.09804 source file (2023-10-12)
Supplement: Supplementary file 1 [file supplement.tex]

%% Math academy 
\begin{table}[ht]
\centering
\begin{tabular}{rrr}
  \hline
 & T=1 & T=2 \\ 
  \hline
I1 & 0.71 & 0.82 \\ 
  I2 & 0.64 & 0.76 \\ 
  I3 & 0.56 & 0.76 \\ 
  I4 & 0.68 & 0.85 \\ 
  I5 & 0.35 & 0.39 \\ 
  I6 & 0.54 & 0.67 \\ 
  I7 & 0.86 & 0.95 \\ 
  I8 & 0.57 & 0.69 \\ 
  I9 & 0.63 & 0.78 \\ 
  I10 & 0.36 & 0.46 \\ 
  I11 & 0.55 & 0.66 \\ 
  I12 & 0.11 & 0.22 \\ 
  I13 & 0.64 & 0.76 \\ 
  I14 & 0.75 & 0.84 \\ 
  I15 & 0.43 & 0.56 \\ 
  I16 & 0.46 & 0.64 \\ 
  I17 & 0.61 & 0.74 \\ 
  I18 & 0.50 & 0.56 \\ 
  I19 & 0.51 & 0.53 \\ 
  I20 & 0.39 & 0.50 \\ 
  I21 & 0.35 & 0.48 \\ 
  I22 & 0.35 & 0.49 \\ 
  I23 & 0.37 &  \\ 
  I24 & 0.20 & 0.26 \\ 
  I25 & 0.19 & 0.19 \\ 
  I26 & 0.54 & 0.63 \\ 
  I27 & 0.57 & 0.61 \\ 
  I28 & 0.36 & 0.51 \\ 
  I29 & 0.44 & 0.54 \\ 
  I30 & 0.81 & 0.91 \\ 
   \hline
\end{tabular}
\end{table}

% NCEDL 

\begin{table}[ht]
\centering
\begin{tabular}{rrr}
  \hline
 & T=1 & T=2 \\ 
  \hline
L1 & 0.58 & 0.80 \\ 
  L2 & 0.59 & 0.85 \\ 
  L3 & 0.56 & 0.92 \\ 
  L4 & 0.45 & 0.87 \\ 
  L5 & 0.55 & 0.90 \\ 
  L6 & 0.26 & 0.74 \\ 
  L7 & 0.23 & 0.79 \\ 
  \hline 
M1 & 0.60 & 0.94 \\ 
  M2 & 0.50 & 0.90 \\ 
  M3 & 0.46 & 0.88 \\ 
  M4 & 0.33 & 0.83 \\ 
  M5 & 0.47 & 0.88 \\ 
  M6 & 0.18 & 0.73 \\ 
  M7 & 0.35 & 0.82 \\   
  
   \hline
\end{tabular}
\end{table}

% Simulation studdy

We conducted a simulation study to evaluate the replicability of estimated model parameters. We considered two assessment  settings that are similar to our two one-topic empirical examples: Scenario 1 considered  $N=750$ and $I=7$, where the average  accuracy rate was 0.3 in Time 1  and 0.8 in Time 2. Scenario 2 considered $N=400$ and $I=30$, where the average  accuracy rate was 0.4 in Time 1  and 0.7 in Time 2. 
We generate 100 datasets in each setting and evaluated the standard deviations of the posterior means of the model parameters. 
Each dataset was analyzed with the one-topic model using the same MCMC setting applied in our empirical examples. 
%Figure xx displays the distributions of the some of the parameters. Other parameter results are presented in the  supplement. 
Table  \ref{tab:sim1} lists the summary of the standard deviations of  the posterior mean estimates across 100 datasets in Scenarios 1 and 2. For  $\lambda_j$, $\theta_j$, and $\beta_i$ parameters, the minimum, maximum, and SD of the standard deviations across the parameters. 
Figures \ref{fg:sim1} and  \ref{fg:sim2} display  the distribution of the posterior mean estimates of some model parameters across 100 replicated datasets under Scenario 1 and 2. 
\textcolor{red}{[other parameters?]}

\begin{table}[hptb]
\centering
\begin{tabular}{cccccc}
  \hline
&  &$\lambda_j$ & $\theta_j$ & $\beta_i$ & $\gamma$ \\ 
  \hline
Scenario 1 & Min & 0.14 & 0.06 & 0.13 & - \\ 
             & Max & 0.22 & 0.10 & 0.14 &  -\\ 
            & Mean & 0.18 & 0.08 & 0.13 &  0.28\\    
             & SD &0.01 & 0.01 & 0.01 &  \\ 
 \hline
Scenario 2  & Min & 0.08 & 0.05 & 0.11 & - \\ 
            &  Max & 0.22 & 0.10 & 0.16 & - \\ 
            &  Mean & 0.17 & 0.07 & 0.13 & 0.14  \\  
            &  SD & 0.03 & 0.01 & 0.01 &  -\\  
   \hline
\end{tabular}
\caption{Summary of the standard deviations of  the posterior mean estimates across 100 datasets  in Scenarios 1 and 2. For  $\lambda_j$, $\theta_j$, and $\beta_i$ parameters, minimum, maximum, and SD of the standard deviations across the parameters.}\label{tab:sim1}
\end{table}

\begin{figure}[hptb]
    \centering
\begin{tabular}{cc}
(a)   & (b)  \\ 
     \includegraphics[width=0.4 \textwidth]{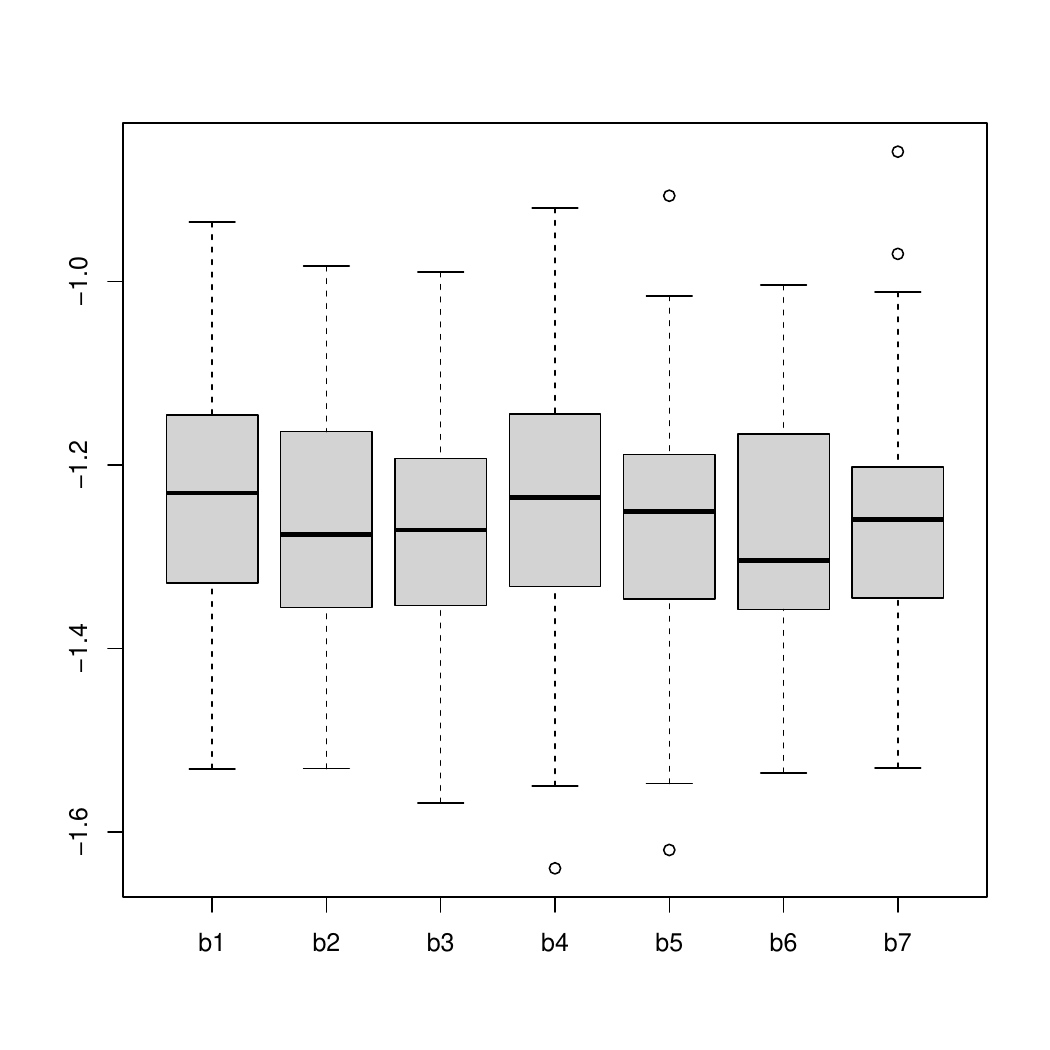} 
     &  \includegraphics[width=0.4 \textwidth]{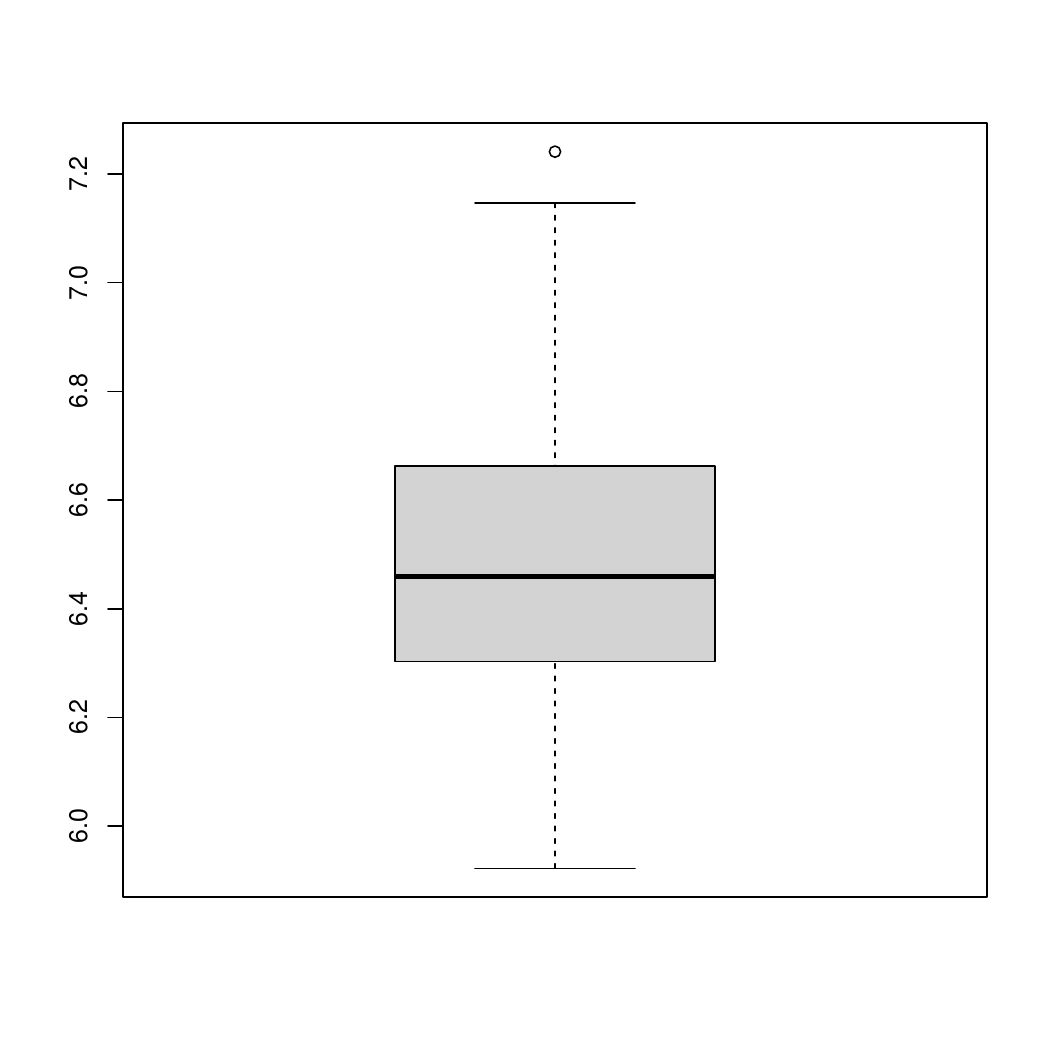}  \\
     \includegraphics[width=0.4 \textwidth]{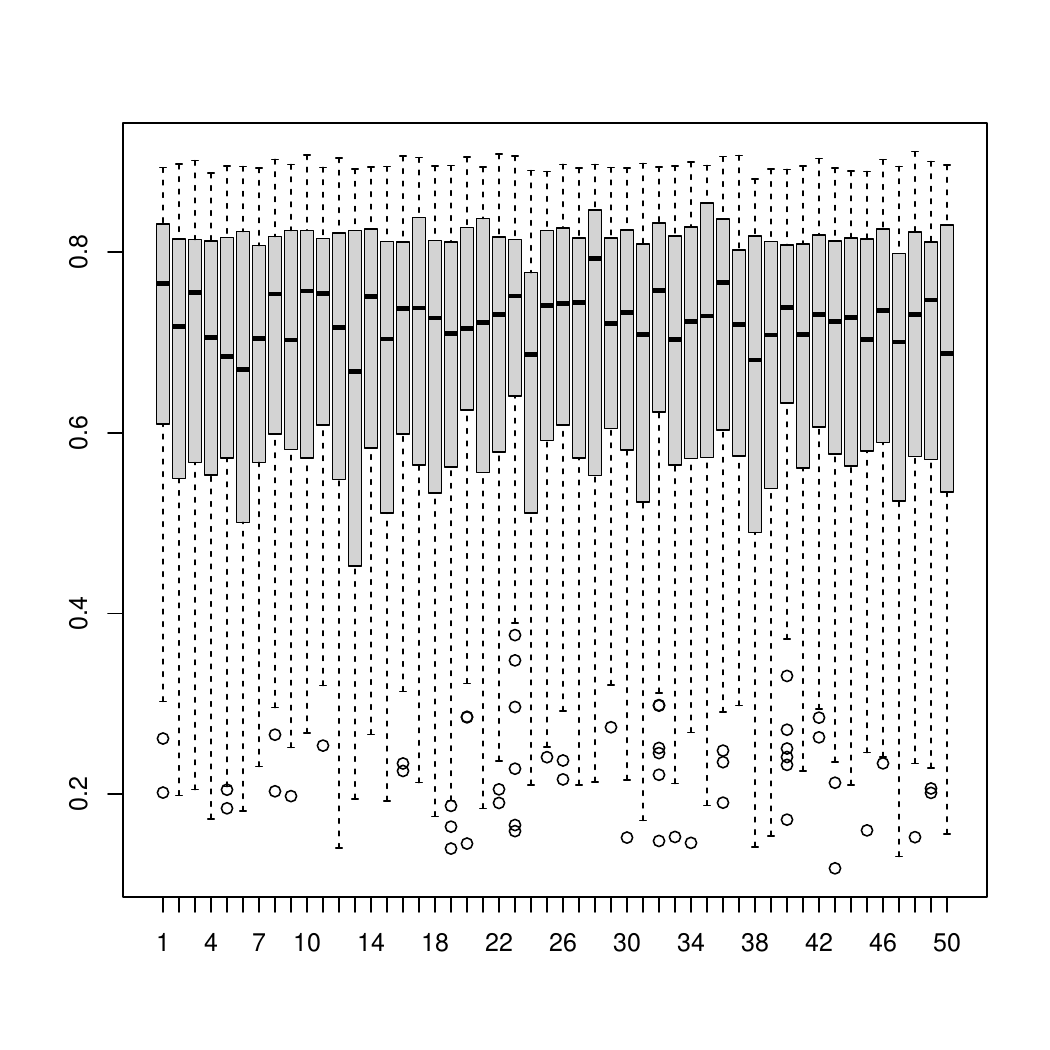} 
     &  \includegraphics[width=0.4 \textwidth]{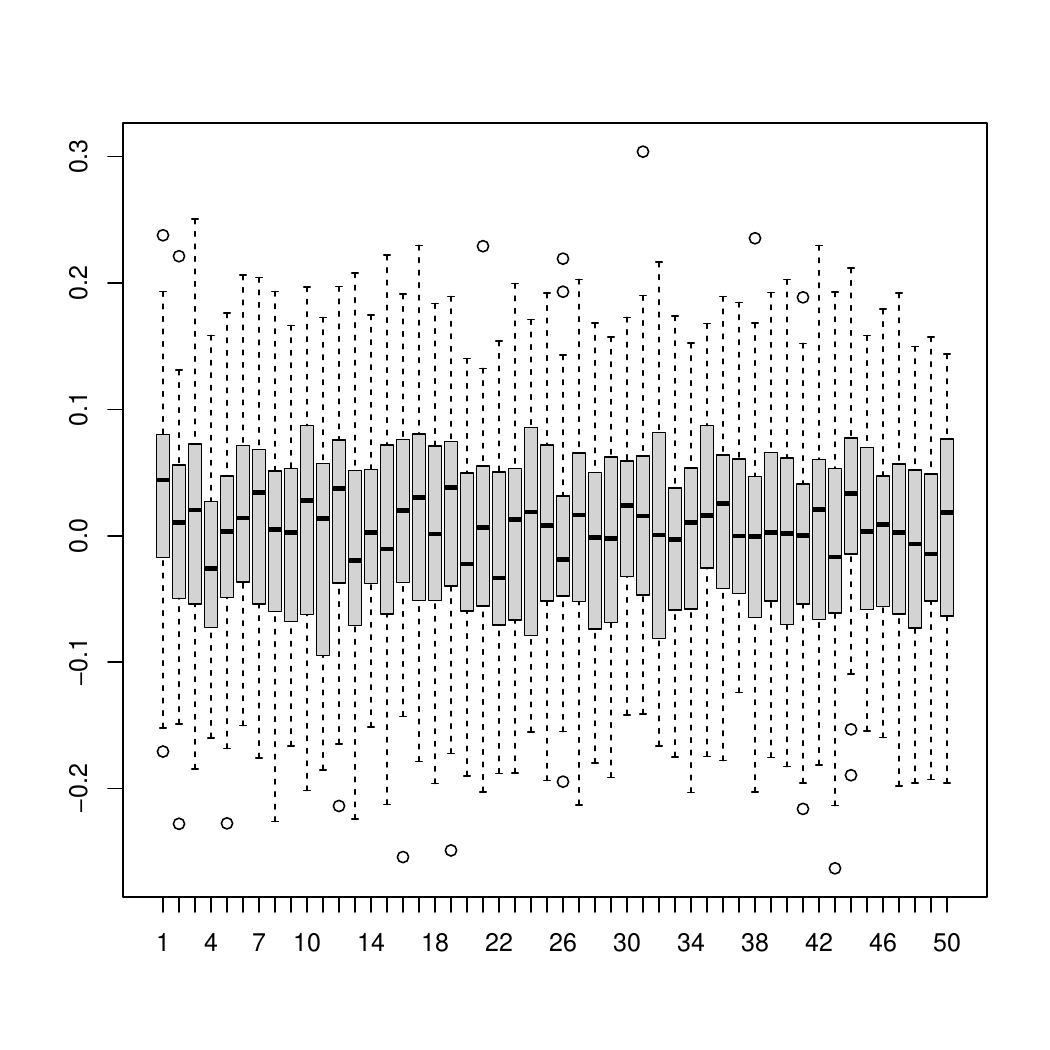}      
\end{tabular}
   \caption{Boxplots of the posterior means of the model parameters across 100 replicated datasets under Scenario 1 } 
   \label{fg:sim1}
\end{figure}

\begin{figure}[hptb]
    \centering
\begin{tabular}{cc}
(a)   & (b)  \\ 
     \includegraphics[width=0.4 \textwidth]{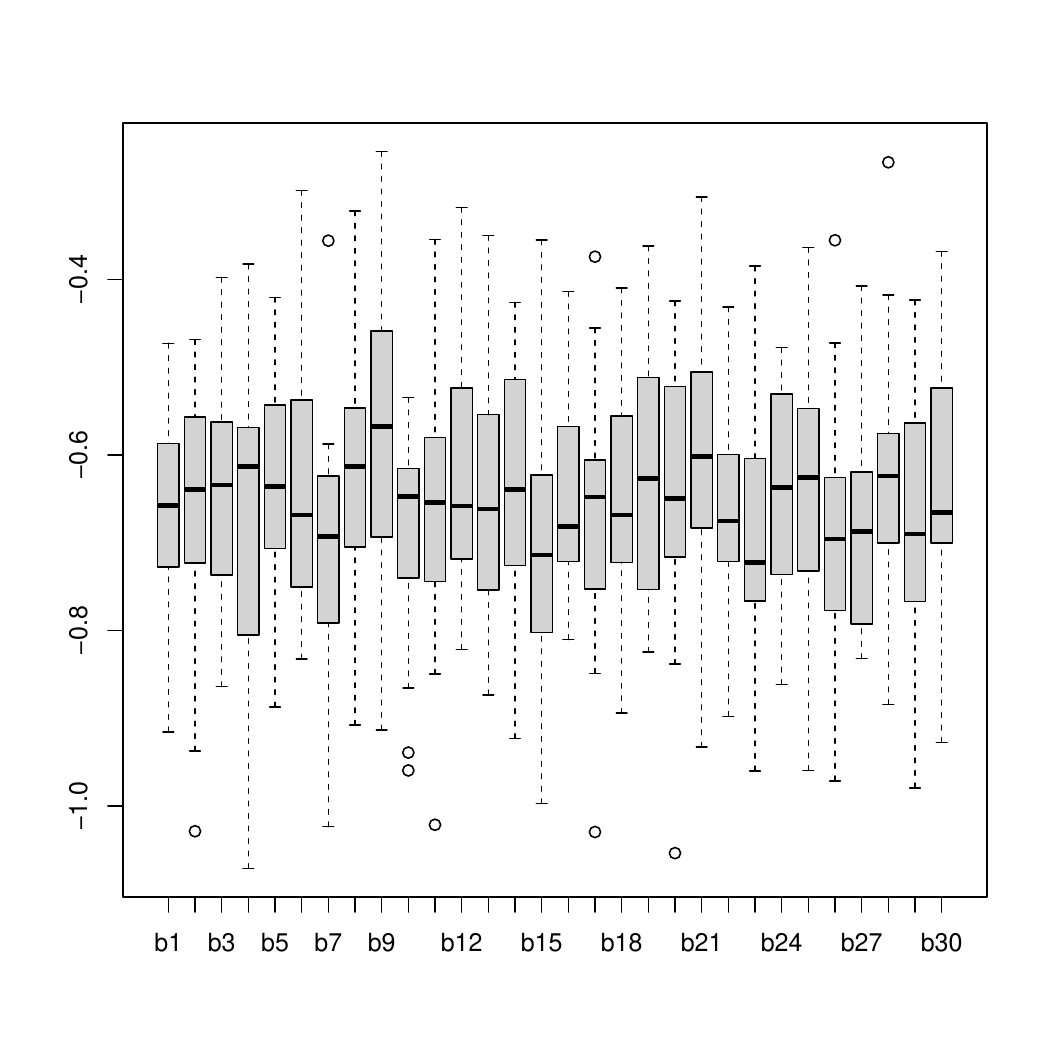} 
     &  \includegraphics[width=0.4 \textwidth]{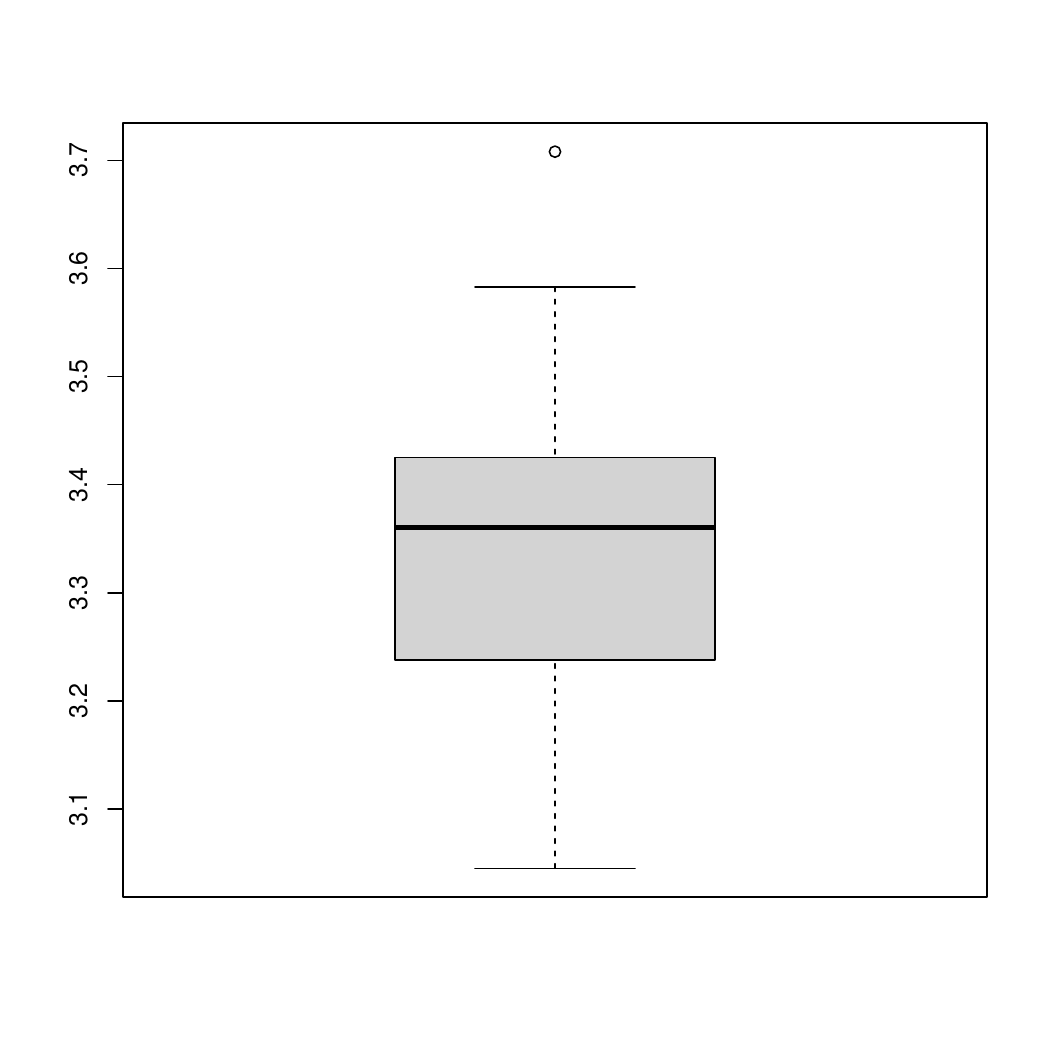}  \\
     \includegraphics[width=0.4 \textwidth]{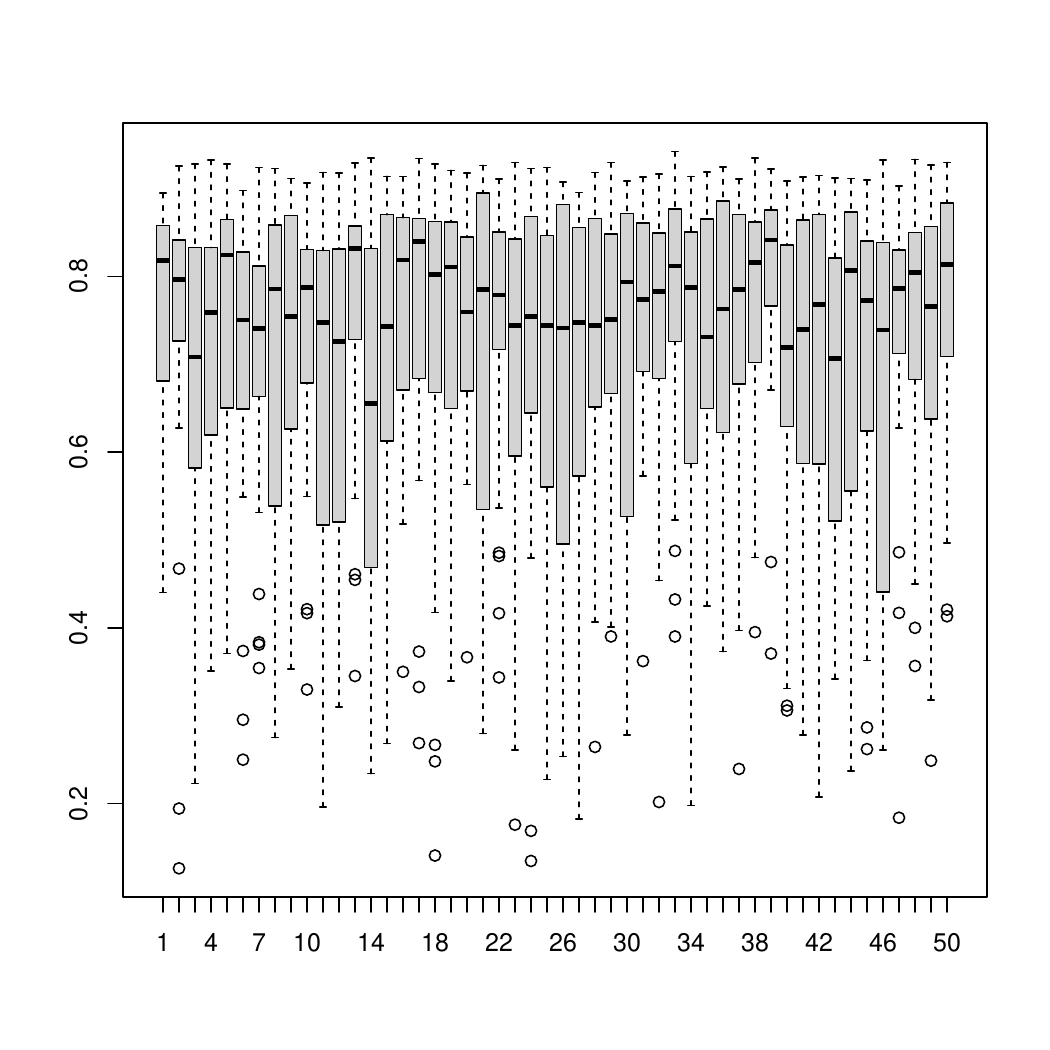} 
     &  \includegraphics[width=0.4 \textwidth]{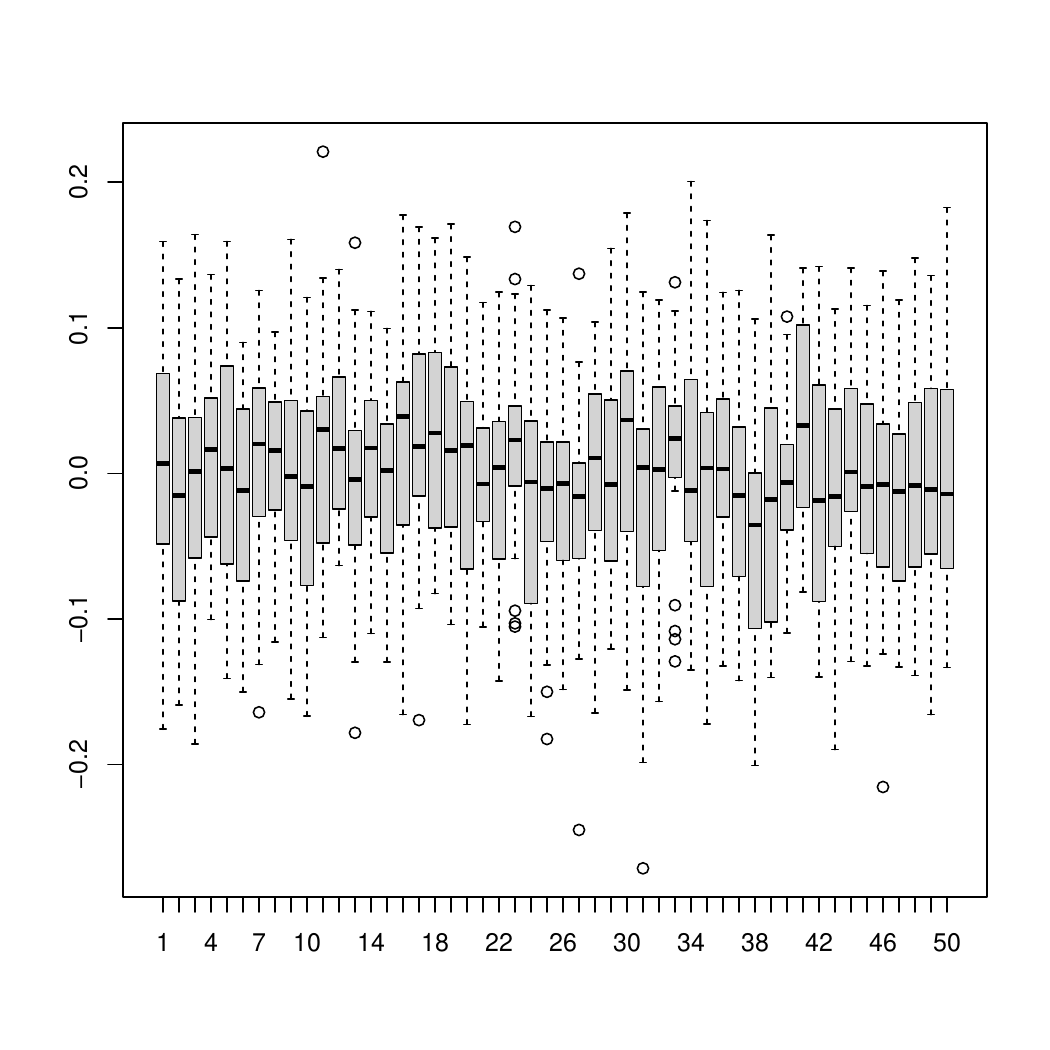}      
\end{tabular}
   \caption{Boxplots of the posterior means of the model parameters across 100 replicated datasets under Scenario 2 } 
   \label{fg:sim2}
\end{figure}
